# Supplementary material for: A fast, large-scale optimal transport algorithm for holographic beam shaping
Source: arXiv:2512.19072 ancillary file (2026-02-19)
Supplement: Supplementary file 1 [file Supplement.pdf]

# A fast, large-scale optimal transport algorithm for holographic beam shaping: Supplementary material

This supplement presents generalizations and implementation details of the algorithms described in the main text. We also provide a basic Julia implementation of the FOT algorithm.

## 1. ARBITRARY LATTICES

For arbitrary input grids and output grids, we require only that the total number of points in each direction coincide for the two. Denoting the number of points in the  $x$  and  $y$  directions as  $n$  and  $m$  respectively, we can thus express the input coordinates as  $x_j = x_0 + j \delta x$ ,  $y_k = y_0 + k \delta y$ ,  $j = 0, \dots, n-1$ ,  $k = 0, \dots, m-1$  and the output coordinates as  $X_J = X_0 + J \Delta X$ ,  $Y_K = Y_0 + K \Delta Y$ ,  $J = 0, \dots, n-1$ ,  $K = 0, \dots, m-1$ .

When using such arbitrary lattices, the object  $\Lambda_{jk}$  used in Sinkhorn-Knopp iterations must be split into two objects  $\Lambda_{jk}^{(x)} = \exp(-(j-K)^2/2n^2\epsilon)$  and  $\Lambda_{jk}^{(y)} = \exp(-(j-K)^2/2m^2\epsilon)$ , and the iterations themselves take the form

$$u_{jk} \leftarrow \frac{g_{jk}^2}{\sum_{LM} \Lambda_{jL}^{(x)} V_{LM} \Lambda_{kM}^{(y)}} = \left[ g^2 \odot \left( \Lambda^{(x)} \cdot V \cdot \Lambda^{(y)} \right) \right]_{jk} \quad (\text{S1})$$

$$V_{JK} \leftarrow \frac{G_{JK}^2}{\sum_{\ell s} \Lambda_{\ell J}^{(x)} u_{\ell s} \Lambda_{sK}^{(y)}} = \left[ G^2 \odot \left( \Lambda^{(x)} \cdot u \cdot \Lambda^{(y)} \right) \right]_{JK}. \quad (\text{S2})$$

Note that we have exploited the fact that  $\Lambda^{(y)}$  is a symmetric matrix in writing the expressions involving matrix multiplication.

We emphasize that while FOT works with such arbitrary lattices, if the input and output grids are not dual in the Fourier sense the discrete Fourier transform will no longer model the physical propagation of light. In this case one must either interpolate fields of one of the input or output lattice onto a grid dual to the other lattice, or else use an alternative method such as a non-uniform discrete Fourier transform to compute the values of a continuous Fourier propagator at non-dual grid points.

For the remainder of this Supplement we generally restrict to the case considered in the main manuscript,  $n = m$ ,  $x_j = y_j = X_j = Y_j = (j - \lfloor n/2 \rfloor) / \sqrt{n}$ .

## 2. LINEAR CONVOLUTION AND CFOT

The linear convolution of two vectors  $x_j$  and  $y_j$ , where  $x$  has indices  $j = p, p+1, \dots, q$  and  $y$  has indices  $j = r, r+1, \dots, s$ , is defined by

$$(x * y)_j := \sum_{k=-\infty}^{\infty} x_{j-k} y_k = \sum_{k=-\infty}^{\infty} x_k y_{j-k} \quad (\text{S3})$$

where we set  $x_j$  and  $y_j$  to zero if  $j$  does not lie in the respective index range  $[p, q]$  or  $[r, s]$ . The equality follows by substituting the summation variable  $k \leftarrow j - k$ . Hereafter we let all unrestricted summations run over all integer values of the summation variable, with any terms with an index out of the respective defined range being set to zero. The linear convolution operation can be implemented with a circular convolution (in which indices are taken modulo the length of the respective vector) by padding both  $x$  and  $y$  with trailing zeros such that they have length at least  $2 \min(q-p, s-r)$ . For a vector  $x_j$  and a matrix  $M_{jk}$ , we define left and right linear convolution in the obvious way

$$(x * M)_{jk} := \sum_{\ell} x_{j-\ell} M_{\ell k} \quad (\text{S4})$$

$$(M * x)_{jk} := \sum_{\ell} M_{j(k-\ell)} x_{\ell}, \quad (\text{S5})$$

which can also be implemented with a circular convolution by zero padding  $x$  and the first or second index of  $M$  as appropriate.

Note that the objects  $\Lambda_{jK} := \exp(-(j-K)^2/2n^2\epsilon)$  and  $\lambda_j := \exp(-j^2/2n^2\epsilon)$  are related by  $\Lambda_{jK} = \lambda_{j-K}$ , which allows us to write

$$(\Lambda \cdot V \cdot \Lambda)_{jk} = \sum_{L,M=0}^{n-1} \Lambda_{jL} V_{LM} \Lambda_{kM} = \sum_{L,M=0}^{n-1} \lambda_{j-L} V_{LM} \lambda_{k-M} = (\lambda * V * \lambda)_{jk}.$$

Note that in programming languages which do not allow negative indexing of vectors, the indices of  $\lambda$  can be taken to run from 0 to  $2n-1$  instead of  $-(n-1)$  to  $n-1$ . In this case, the above relation becomes

$$(\Lambda \cdot V \cdot \Lambda)_{jk} = (\lambda * V * \lambda)_{(j+n-1)(k+n-1)}, \quad (\text{S6})$$

thus requiring an offset of the index of the latter array.

Our implementation of cFOT uses zero padding and circular convolutions to apply linear convolution. There are a variety of other methods for accomplishing Gaussian convolutions [1] which differ significantly in speed and accuracy. Of greatest relevance to the cFOT algorithm, one would like a convolution method which allows stable performance at smaller  $\epsilon$  values (see Section 3) and/or which is significantly faster. We have not identified an alternative to padding and circular convolution which improves stability at low  $\epsilon$ , and we have realized improved speed only at a significant penalty with regard to  $\epsilon$  stability. We have not exhaustively optimized this aspect of our cFOT implementation, however, and improved performance of this algorithm may well be possible.

### 3. EPSILON INSTABILITY

Numerical instability can occur for very small values of the regularization parameter  $\epsilon$ . This effect is due to division by small numbers in Eqs. (S1) and (S2), and can eventually result in numerical overflow (floating point value NaN) in  $u$  and  $V$ . Once a single such value is present, typically the entire array will be populated with NaNs within one or two iterations, and no useful information can be obtained from the solution.

This effect can be mitigated somewhat by identifying points in  $\Lambda \cdot V \cdot \Lambda$  which are too small to be reliably inverted and setting the inverse of these points to zero instead. This can prevent  $u$  and  $V$  from becoming populated entirely by NaN, and thus allow for slightly lower values of  $\epsilon$  to be used. However, the resulting rounding errors tend to compromise the accuracy of phase solutions, and so it is generally not advisable to push  $\epsilon$  much lower than would otherwise generate floating point overflow.

Several methods for improving stability of Sinkhorn iterations at low  $\epsilon$  have been proposed [2, 3], though that of [2] may compromise the memory scaling advantage which is central to the FOT algorithm. Our experimentation with  $\epsilon$  scheduling (as in [3]) has allowed stable iteration at slightly lower values of  $\epsilon$ , but we do not see a significant benefit for overall performance of FOT.

### 4. LOSS FUNCTIONS AND CONVERGENCE

Loss functions serve two purposes in the context of beam shaping. The first is to assess the quality of a phase solution. The second is to establish whether an iterative solution algorithm has converged. Different loss functions have different roles in fulfilling these two goals.  $L^p$  and RMS loss functions are typically a reasonable model of what is desired of a phase solution experimentally, and thus serve well for the first objective.  $L^p$  intensity loss is defined by

$$L_I^p(\phi, g, G) := \sum_{LM} \left| \left| \mathcal{F} \left[ g_{jk} e^{2\pi i \phi_{jk}} \right]_{LM} \right|^2 - G_{LM}^2 \right|^p, \quad (\text{S7})$$

where  $\mathcal{F}$  denotes the discrete Fourier transform and we assume that the input and output grids are Fourier dual to each other so that we may use  $\mathcal{F}$  to implement light propagation between the two domains.  $L^p$  amplitude loss is very similar to  $L^p$  intensity loss, being defined by

$$L_A^p(\phi, g, G) := \sum_{LM} \left| \left| \mathcal{F} \left[ g_{jk} e^{2\pi i \phi_{jk}} \right]_{LM} \right| - G_{LM} \right|^p. \quad (\text{S8})$$

RMS intensity loss is defined with respect to a region of interest  $R$  in the output lattice, represented as a subset of the grid indices  $\{(J, K) : J \in \{0, \dots, n-1\}, K \in \{0, \dots, m-1\}\}$ , which

is intended to capture the portion of the target beam for which we care about the quality of the output. It has the definition

$$L_{RMS}(\phi, g, G) := \sqrt{\frac{1}{|R|} \sum_{(J,K) \in R} \frac{(\tilde{G}_{JK}^2 - \hat{G}_{JK}^2)^2}{\hat{G}_{JK}^4}}, \quad (S9)$$

where

$$\tilde{G}_{JK} = \frac{\mathcal{F} [g_{jk} e^{2\pi i \phi_{jk}}]_{JK}}{\sqrt{\sum_{(L,M) \in R} \mathcal{F} [g_{jk} e^{2\pi i \phi_{jk}}]_{LM}^2}} \quad (S10)$$

$$\hat{G}_{JK} = \frac{G_{JK}}{\sqrt{\sum_{(L,M) \in R} G_{LM}^2}} \quad (S11)$$

are the output beam and target beam, respectively, renormalized over the region of interest  $R$ .

Any of  $L_I^p$ ,  $L_A^p$ , or  $L_{RMS}$  are reasonable ways to gauge the quality of a phase solution, and many of these losses are rigorously bounded by each other. We have used  $L_I^1$  for our assessment of the FOT algorithm due to its simplicity.

For the purposes of evaluating the convergence of the Sinkhorn-Knopp algorithm, a more natural choice of loss is the marginal constraint violation,

$$L_{CV}(u, V, g, G) = \sum_{jk} |g_{jk}^2 - u_{jk}(\Lambda^{(x)} \cdot V \cdot \Lambda^{(y)})_{jk}| + \sum_{JK} |G_{JK}^2 - V_{JK}(\Lambda^{(x)} \cdot u \cdot \Lambda^{(y)})_{JK}|. \quad (S12)$$

This function can be computed in the loop of the FOT algorithm, by reusing the results of  $\Lambda^{(x)} \cdot V \cdot \Lambda^{(y)}$  and  $\Lambda^{(x)} \cdot u \cdot \Lambda^{(y)}$ . It has been shown in [4] that Sinkhorn-Knopp iterations have guaranteed convergence with respect to  $L_{CV}$ . This loss can be interpreted as twice the total variation distance [5] between the marginals of the transport plan defined by  $u$  and  $V$  and the desired marginals  $g^2$  and  $G^2$ .

## 5. REQUIRED NUMBER OF ITERATIONS

It has been shown in [4] that Sinkhorn-Knopp requires  $\mathcal{O}(\delta^{-2} \log(s/l))$  iterations to converge to a tolerance  $\delta$  with respect to the total variation metric of Eq. (S12), where  $l$  and  $s$  are defined in terms of the array  $A_{jkLM} = \exp(-c_{jkLM}/\epsilon)$  by  $l = \min_{jkLM} A_{jkLM}$  and  $s = \sum_{jkLM} A_{jkLM} = \sum_{jL} \Lambda_{jL} \Lambda_{kM} = (\sum_{jL} \Lambda_{jL}) (\sum_{kM} \Lambda_{kM})$ . Evaluating  $l$  for our cost matrix yields

$$l = \min_{jLkM} A_{jkLM} = \exp\left(-\frac{(n-1)^2}{n^2\epsilon}\right) = e^{-1/\epsilon} + \mathcal{O}(1/n). \quad (S13)$$

To evaluate  $s$ , we interpret  $\sum_{jL} \Lambda_{jL}$  as a Riemann sum. Setting  $x = j/n$  and  $y = L/n$ , we find:

$$\begin{aligned} \sum_{jL} \Lambda_{jL} &= \sum_{j=0}^{n-1} \sum_{L=0}^{n-1} \exp(-(j-L)^2/(2n^2\epsilon)) = n^2 \int_0^1 dx \int_0^1 dy \exp(-(x-y)^2/(2\epsilon)) + \mathcal{O}(n) \quad (S14) \\ &= n^2 \left[ \sqrt{2\pi\epsilon} \operatorname{Erf}\left(\frac{1}{\sqrt{2\epsilon}}\right) + 2\epsilon(e^{-\epsilon/2} - 1) \right] + \mathcal{O}(n) \quad (S15) \end{aligned}$$

which implies that  $s$  is  $\mathcal{O}(n^4)$ . Combining these results, we obtain that the required number of iterations is indeed  $\mathcal{O}(\delta^{-2} \log(s/l)) = \mathcal{O}(\delta^{-2} \log(n^4))$ , or equivalently  $\mathcal{O}(\delta^{-2} \log(N))$ , as was stated in the main text.

Note that this bound is irrespective of the particular input or target beam profiles, though in practice we find that convergence is faster for simpler shapes.

## 6. EXAMPLE JULIA CODE

Below we present a basic Julia 1.11.7 implementation of the FOT algorithm. For a packaged implementation with other supporting tools, see [6].

```
1 function natrange(n::Int)
2     return (-floor(n / 2):floor((n - 1) / 2)) ./ sqrt(n)
3 end
4
5 function natlat(ns::NTuple{N,Integer}) where {N}
6     return ((natrange(n) for n in ns)...,)
7 end
8
9 function integrate_phase(
10     dphi_dx::Matrix{Float64},
11     dphi_dy::Matrix{Float64}
12 )
13     @assert size(dphi_dx) == size(dphi_dy) "
14         dphi_dx and dphi_dy must have the same size"
15
16     # precompute constants
17     Nx, Ny = size(dphi_dx)
18     dx, dy = 1/sqrt(Nx), 1/sqrt(Ny)
19     x0, y0 = div(Nx,2), div(Ny,2)
20
21     # trapezoid integration
22     # integrate along (x0, y0)->(x,y0)
23     Ix = cumsum(dphi_dx[:,y0]) - dphi_dx[:,y0] ./ 2
24     Ix .-= Ix[x0]
25     # integrate along (x, y0)->(x,y)
26     Iy = cumsum(dphi_dy, dims=2) - dphi_dy / 2
27     Iy .-= Iy[:,y0]
28     # final phase
29     phi = Ix * dx .+ Iy * dy
30     return phi
31 end
32
33 function fot(
34     inputIntensity::Matrix{Float64},
35     targetIntensity::Matrix{Float64};
36     epsilon::Float64=0.0002,
37     ot_iter::Int=200
38 )
39     @assert size(inputIntensity) == size(targetIntensity) "
40         inputIntensity and targetIntensity must have the same size"
41     a = inputIntensity ./ sum(inputIntensity)
42     b = targetIntensity ./ sum(targetIntensity)
43     n,m = size(a)
44     X, Y = natlat((n,m))
45     Kx = [exp(-(i - j)^2/(2*n*epsilon)) for i in X, j in X]
46     Ky = [exp(-(i - j)^2/(2*n*epsilon)) for i in Y, j in Y]
47     u = fill(1/(n*m), (n,m))
48     v = fill(1/(n*m), (n,m));
49
50     # Sinkhorn-Knopp iteration
51     for iter in 1:ot_iter
52         u = a ./ (Kx * v * Ky)
53         v = b ./ (Kx * u * Ky)
54     end
55
```

```

56     # gradients
57     scale = u ./ a
58     dphi_dx = scale .* (Kx * (v .* X) * Ky)
59     dphi_dy = scale .* (Kx * (v .* Y') * Ky)
60
61     # Integrate dphi_dx and dphi_dy to get the final phase
62     phi = integrate_phase(dphi_dx, dphi_dy)
63     return phi
64 end

```

#### A. Example Usage

An example of the usage of the above Julia implementation of FOT is the following.

```

1  using Images, FFTW
2
3  function look(f::AbstractArray{T,N}) where {T<:Real,N}
4      return Gray.(f ./ maximum(f))
5  end
6  function look(x...)
7      return hcat([look(y) for y in x]...)
8  end
9  function shifted_fft(field)
10     N = prod(size(field))
11     return fftshift(fft(ifftshift(field))) / sqrt(N)
12 end
13 function inv_shifted_fft(field)
14     return fftshift(ifft(ifftshift(field)))
15 end
16
17 n,sigma,R,w = 1024,15,8,2
18 L = natrange(n)
19
20 g = [exp(-(x^2+y^2)/(2sigma)) for x in L, y in L]
21 G = [exp(-(sqrt(x^2+y^2)-R)^2/(2w)) for x in L, y in L]
22 phi = fot(g.^2,G.^2)
23 look(g,G,abs.(shifted_fft(g.*exp.(2pi*im*phi))))

```

#### REFERENCES

1. P. Getreuer, “A survey of gaussian convolution algorithms,” *Image Process. On Line* **2013**, 286–310 (2013).
2. B. Schmitzer, “Stabilized sparse scaling algorithms for entropy regularized transport problems,” *SIAM J. on Sci. Comput.* **41**, A1443–A1481 (2019).
3. J. Chen, L. Chen, Y. P. Liu, *et al.*, “Exponential convergence of sinkhorn under regularization scheduling,” in *SIAM Conference on Applied and Computational Discrete Algorithms (ACDA23)*, (SIAM, 2023), pp. 180–188.
4. J. Altschuler, J. Niles-Weed, and P. Rigollet, “Near-linear time approximation algorithms for optimal transport via sinkhorn iteration,” *Adv. neural information processing systems* **30** (2017).
5. A. B. Tsybakov, *Introduction to Nonparametric Estimation* (Springer, New York, NY, 2009).
6. H. Swan, M. Van de Graaff, and A. Torchilo, “SLMTools,” <https://github.com/hoganphysics/SLMTools>, commit: d7db9fd (2025).
